# Supplementary material for: Agent57: Outperforming the Atari Human Benchmark
Source: arXiv:2003.13350 source file (2020-03-30)
Supplement: Supplementary file 1 [file computational_analysis.tex]

\section{Computational analysis}
\subsection{Algorithm Computation comparison}
For all the ablations done on $10$ Atari games, we run and report our results after the actors of Agent57 have consumed $50$ billion frames in total.

In Tab. \ref{table_computation_comparison} we detail the number of steps used by the algorithms used on the $57$ Atari games. All algorithms use $256$ except MuZero, for which this information is not described in the work. The agents are stopped when they hold a similar score for $5$ billion frames. Also, we note that the best performing agent, R2D2(bandit), was run for the same number of steps as Agent57, to ensure that results are comparable.

\begin{table}
\begin{tabular}{l|cccccc}
Algorithm & Agent57 & R2D2(bandit) & R2D2 & NGU & R2D2 Retrace & MuZero \\ \hline
Total Number of frames & $90$ B & $90$ B & $70$ B & $45$ B & $45$ B & $20$ B
\end{tabular}

\caption{Computation comparison.}
\label{table_computation_comparison}
\vspace{-2ex}
\end{table}

\subsection{Complexity analysis}
The number of weights that the network has can be computed from the sizes of the architecture seen in App. \ref{app:neural}. Also, as done in NGU, at the beginning of training, we pre-allocate the memory that the episodic memory buffer of the intrinsic motivation uses. Both of these statements imply that the space complexity is constant.

Regarding time complexity, we use no more computation than NGU: that is, we perform a forward pass per frame we observe, and also we compute the intrinsic reward at every time step. To do that, we compute the distance from the embeddings produced by the inverse dynamics model of NGU to the contents of the episodic memory in order to retrieve the $k$-nearest neighbors. Therefore, time complexity is $O(M\cdot N)$, where $N$ is the number of frames, and $M$ is the size of our memory.
